# Supplementary material for: Cross-Document Contextual Coreference Resolution in Knowledge Graphs
Source: arXiv:2504.05767 source file (2025-04-08)
Supplement: Supplementary file 1 [file appendix.tex]

\section{Contextual Embeddings Utilization}

The exploration of contextual embeddings plays a pivotal role in enhancing coreference resolution across multiple documents within knowledge graphs. The methodology we propose integrates various contextual embedding approaches to optimize performance metrics, specifically precision, recall, and F1 Score. Table~\ref{tab:contextual_embeddings} illustrates the comparative effectiveness of different models utilizing distinct contextual embeddings for resolving coreferences.

\textbf{Contextual embeddings significantly influence coreference resolution accuracy.} Among the evaluated models, ThaiCoref utilizing GloVe embeddings demonstrates the highest performance with a precision of 78.0\%, a recall of 76.5\%, and an F1 Score of 77.2\%. This indicates that GloVe effectively captures the semantic relationships pertinent to coreference resolution tasks. Following closely is Llama-3 with BERT-based embeddings, which presents a precision of 75.5\% and a recall of 73.0\%, yielding an F1 Score of 74.2\%. In contrast, CorefUD with ELMo embeddings shows relatively lower performance, with metrics registering at a precision of 68.6\% and a recall of 65.0\%. 

These results signify that the choice of contextual embedding has a direct effect on the model's capacity to accurately resolve coreferences. It is evident from the results that advanced models employing sophisticated contextual embeddings outperform those relying on simpler embeddings, indicating the enhancement in understanding inter-document relationships facilitated by structured knowledge representations. This underlines the imperative of selecting appropriate embeddings to optimize coreference resolution methodologies within knowledge graph contexts.

\section{Graph-Based Inference Techniques}

\begin{figure}[tp]
    \centering
    \includegraphics[width=1\linewidth]{figure2.png}
    \caption{Evaluation of graph-based inference techniques used in coreference resolution models, including accuracy, processing time, and memory consumption.}
    \label{fig:figure2}
\end{figure}

\begin{table}[tp]
\resizebox{\linewidth}{!}{
\begin{tabular}{lccccc}
\toprule
\textbf{Model} & \textbf{Contextual Embedding} & \textbf{Precision} & \textbf{Recall} & \textbf{F1 Score} \\ \midrule
Llama-3        & BERT-based                   & 75.5               & 73.0            & 74.2               \\
GPT-3.5        & RoBERTa                      & 72.3               & 70.1            & 71.2               \\
CorefUD        & ELMo                         & 68.6               & 65.0            & 66.7               \\
ThaiCoref      & GloVe                        & 78.0               & 76.5            & 77.2               \\
Major Entity ID & FastText                    & 65.4               & 63.2            & 64.3               \\ \bottomrule
\end{tabular}}
\caption{Evaluation of different contextual embeddings on coreference resolution performance metrics.}
\label{tab:contextual_embeddings}
\end{table}

The exploration of graph-based inference techniques reveals their critical role in enhancing coreference resolution across multiple documents. As shown in Figure~\ref{fig:figure2}, various models demonstrate differing levels of effectiveness based on the type of graph utilized.

\textbf{Contextual Graphs yield the highest inference accuracy.} The results indicate that the Llama-3 model, utilizing a Contextual Graph, achieves an impressive accuracy of 85.2\%, showcasing its ability to effectively resolve coreferences. In comparison, the Event Coref Bank Plus, with a Dynamic Graph structure, boasts the highest accuracy at 86.5\%, emphasizing the advantages of dynamic linking in understanding complex inter-document relationships.

\textbf{Processing time and memory usage efficiency are essential metrics to consider.} Llama-3 processes coreferences in 2.5 seconds and uses 120 MB of memory, making it relatively efficient among the models assessed. On the other hand, CorefUD shows a longer processing time of 3.0 seconds and lower memory consumption at 95 MB, which signals that variations in graph design can significantly impact both time efficiency and resource utilization.

\textbf{The trade-offs between models are evident.} While the GPT-3.5 model with an Entity Graph has robust accuracy at 83.1\%, it requires 2.8 seconds and 110 MB of memory, highlighting a balance between computational efficiency and performance. In the case of Major Entity Identification, although the accuracy is lower at 78.9\%, it still maintains a reasonable processing time of 3.1 seconds, illustrating that not all models sacrifice performance for efficiency.

\section{Dynamic Linking Mechanism}

\begin{table}[tp]
\resizebox{\linewidth}{!}{
\begin{tabular}{lcccccc}
\toprule
\textbf{Model}          & \textbf{Dataset} & \textbf{Linking Precision} & \textbf{Linking Recall} & \textbf{Linking F1} \\ \midrule
\textbf{Llama-3}       & SP-10K          & 73.5                     & 70.2                    & 71.8                  \\
                      & CoNLL-2012       & 76.2                     & 74.0                    & 75.1                  \\ \midrule
\textbf{GPT-3.5}      & ConceptNet      & 71.0                     & 68.1                    & 69.5                  \\
                      & Complex SQ      & 75.2                     & 72.4                    & 73.8                  \\ \midrule
\textbf{CorefUD}      & LexGLUE        & 67.8                     & 64.5                    & 66.1                  \\
                      & GLUE           & 69.3                     & 66.2                    & 67.8                  \\ \midrule
\textbf{ThaiCoref}    & SP-10K         & 79.1                     & 77.0                    & 78.1                  \\
                      & CoNLL-2012      & 81.0                     & 79.5                    & 80.2                  \\ \midrule
\textbf{Major Entity Identification} & ConceptNet      & 64.5                     & 62.0                    & 63.2                  \\
                      & Complex SQ      & 65.8                     & 64.0                    & 64.9                  \\ \midrule
\textbf{Event Coref Bank Plus} & LexGLUE        & 67.5                     & 66.0                    & 66.8                  \\
                      & GLUE           & 71.1                     & 70.0                    & 70.5                  \\ \midrule
\textbf{Rationale-centric Approach} & SP-10K         & 76.0                     & 74.3                    & 75.1                  \\
                      & CoNLL-2012      & 77.5                     & 75.4                    & 76.4                  \\ \bottomrule
\end{tabular}}
\caption{Evaluation of the dynamic linking mechanism across various models on coreference resolution datasets.}
\label{tab:linking_performance}
\end{table}

The dynamic linking mechanism introduced for coreference resolution in knowledge graphs highlights the advantages of structured knowledge representations when addressing references to the same entities across multiple documents. Table~\ref{tab:linking_performance} presents a detailed evaluation of various models, illustrating their performance across different datasets concerning linking precision, recall, and F1 scores.

\textbf{Llama-3 demonstrates strong performance, particularly on CoNLL-2012, achieving a linking precision of 76.2\% and recall of 74.0\%.} This showcases its effectiveness in accurately identifying coreferences when leveraging contextual embeddings and sophisticated graph-based inference techniques. 

\textbf{GPT-3.5 shows reasonable performance across datasets, with its highest F1 score of 73.8\% on the Complex SQ dataset.} The linking precision and recall metrics highlight a robust understanding of entity references, although slightly lower than Llama-3.

\textbf{ThaiCoref indicates the best performance among all the models, with linking precision peaking at 81.0\% on CoNLL-2012.} This implies that ThaiCoref effectively manages intricate relationships within the datasets, leading to superior recall metrics as well.

This assessment underscores the efficacy of the dynamic linking approach in enhancing coreference resolution, indicating that more sophisticated mechanisms can lead to significant improvements in entity linking tasks across various applications.
